# Supplementary material for: A Flexible Model for Record Linkage
Source: arXiv:2407.06835 source file (2025-09-15)
Supplement: Supplementary file 2 [file Simplistic_SHIW.tex]

\begin{tikzpicture}[x=1pt,y=1pt]
    \begin{axis}[
        xmin=-0.05, xmax=0.45,
        ymin=0, ymax=1,
        xtick={0,0.1,0.2,0.3,0.4},
        ytick={0,0.2,0.4,0.6,0.8,1},
        legend style={at={(0.9,0.59)}},
        legend entries={F1-Score, FDR, Sensitivity} ]
    \addplot[smooth,dashed] plot coordinates { (0.04,0.35)
        (0.12,0.30)
        (0.19,0.25)
        (0.27,0.20)
        (0.34,0.16)
        (0.40,0.12) };
    \addplot[smooth] plot coordinates { (0.04,0.76)
        (0.12,0.78)
        (0.19,0.80)
        (0.27,0.83)
        (0.34,0.86)
        (0.40,0.88) };
    \addplot[smooth,dotted] plot coordinates { (0.04,0.67)
        (0.12,0.49)
        (0.19,0.35)
        (0.27,0.24)
        (0.34,0.18)
        (0.40,0.13) };
    \end{axis}
\end{tikzpicture}
