# Supplementary material for: A Flexible Model for Record Linkage
Source: arXiv:2407.06835 source file (2025-09-15)
Supplement: Supplementary file 3 [file perf_distortion_SHIW.tex]

\begin{figure}[!h]
    \centering
    \begin{tikzpicture}
    \node at (0.3,-5.55) {\textit{FlexRL}};
    \node at (7.8,-5.55) {Simplistic};
    \node at (0,-7.85) {\scalebox{0.7}{\input{Figures/FigSuppl_Distortion/FlexRL_SHIW}}};
    \node at (7.5,-7.85) {\scalebox{0.7}{\input{Figures/FigSuppl_Distortion/Simplistic_SHIW}}};
    \node at (4.1,-10.3) {Distortion};
    \end{tikzpicture}
    \caption{Evolution of the F1-score, FDR and sensitivity for screwed versions of the complete SHIW data sets. We artificially distort the data and we define the distortion level (x-axis) as the sum of medians of disagreements and missing values among the PIVS of true links.}
    \label{fig_performancesXdeformationsSHIW}
\end{figure}
