# Supplementary material for: A Flexible Model for Record Linkage
Source: arXiv:2407.06835 source file (2025-09-15)
Supplement: Supplementary file 4 [file histogram_linkage_proba.tex]

\begin{figure}
    \centering
    \begin{tikzpicture}
    \begin{axis}[
        ymin=0, ymax=10,
        ytick={0,2,4,6,8,10},
        yticklabels={$\log_{10} 10^{0\hphantom{0}}$, $\log_{10} 10^{2\hphantom{0}}$, $\log_{10} 10^{4\hphantom{0}}$, $\log_{10} 10^{6\hphantom{0}}$, $\log_{10} 10^{8\hphantom{0}}$, $\log_{10} 10^{10}$} 
        ]
    \addplot+[ybar interval, mark=no, draw=black
    ] plot coordinates { (0, 8.39) (0.05, 3.80) (0.1, 3.64) (0.15, 3.50) (0.2, 3.39) (0.25, 3.30) (0.3, 3.19) (0.35, 3.10) (0.4, 3.02) (0.45, 2.96) (0.5, 2.89) (0.55, 2.83) (0.6, 2.75) (0.65, 2.73) (0.7, 2.66) (0.75, 2.67) (0.8, 2.64) (0.85, 2.62) (0.9, 2.68) (0.95, 3.64) (1, 3.64) };
    \end{axis}
    \end{tikzpicture}
    \caption{Linkage probabilities in \smash{$\boldsymbol{\hat\Delta}$} on a log (base 10) scale for the SHIW data sets. The bimodal distribution is representing the mixture between links and non links (and uncertain cases in between).}
    \label{fig_SHIWprobaDeltaHist}
\end{figure}
