# Supplementary material for: A Flexible Model for Record Linkage
Source: arXiv:2407.06835 source file (2025-09-15)
Supplement: Supplementary file 5 [file Boxplots_SHIW.tex]

\begin{figure}[!h]
    \centering
    \begin{tikzpicture}
    \node at (0.3,-5.27) {F1-Score};
    \node at (5.8,-5.27) {False Discovery Rate};
    \node at (11.3,-5.27) {Sensitivity};
    \node at (0,-7.85) {\scalebox{0.7}{\input{Figures/FigSuppl_Regional_Boxplots_SHIW/F1Score_SHIW}}};
    \node at (5.5,-7.85) {\scalebox{0.7}{\input{Figures/FigSuppl_Regional_Boxplots_SHIW/FDR_SHIW}}};
    \node at (11,-7.85) {\scalebox{0.7}{\input{Figures/FigSuppl_Regional_Boxplots_SHIW/Sensitivity_SHIW}}};
    \end{tikzpicture}
    \caption{Boxplots showing the variability of the F1-score, the FDR and the sensitivity of the compared methods on regional subsets of the SHIW data sets: Piedmont, Aosta Valley, Lombardy, Trentino-Alto Adige, Veneto, Friuli–Venezia Giulia, Liguria, Emilia–Romagna, Tuscany, Umbria, Marche, Lazio, Abruzzo, Molise, Campania, Apulia, Basilicata, Calabria, Sicily, Sardinia.}
    \label{fig_Regional_Boxplots_SHIW}
\end{figure}
