# Supplementary material for: A Flexible Model for Record Linkage
Source: arXiv:2407.06835 source file (2025-09-15)
Supplement: Supplementary file 6 [file F1Score_SHIW.tex]

\begin{tikzpicture}[x=1pt,y=1pt]
      \begin{axis}
        [
        boxplot/draw direction=y,
        ymin=0,ymax=1,
        xtick={1,2,3,4},
        xticklabels={\textit{FlexRL}, \textit{Exchanger}, \textit{BRL}, Simplistic},
        cycle list={{black},{black},{black},{black}}
        ]
        \addplot+[mark = o,
        boxplot prepared={
          lower whisker  =0.1775,
          lower quartile =0.3588,
          median         =0.3875,
          upper quartile =0.5544,
          upper whisker  =0.7826
        },
        ] coordinates {(0,0.3649123)(0,0.7826087)(0,0.3698469)(0,0.3585434)(0,0.2727273)(0,0.5629630)(0,0.5902778)(0,0.3591549)(0,0.3747981)(0,0.4587525)(0,0.5458613)(0,0.3800384)(0,0.4695652)(0,0.7567568)(0,0.2240326)(0,0.2282794)(0,0.6878307)(0,0.4744526)(0,0.1775148)(0,0.3949580)};
        \addplot+[mark = o,
        boxplot prepared={
          lower whisker  =0.0693,
          lower quartile =0.0955,
          median         =0.1607,
          upper quartile =0.2837,
          upper whisker  =0.4875
        },
        ] coordinates {(0,0.07858688)(0,0.57777780)(0,0.07016992)(0,0.10763640)(0,0.10509140)(0,0.25423730)(0,0.31319910)(0,0.09767092)(0,0.14671420)(0,0.19984740)(0,0.23725060)(0,0.11382110)(0,0.35409840)(0,0.48745520)(0,0.09333850)(0,0.06933020)(0,0.38805970)(0,0.22845690)(0,0.07900751)(0,0.17469390)};
        \addplot+[mark = o,
        boxplot prepared={
          lower whisker  =0.0771,
          lower quartile =0.1702,
          median         =0.3537,
          upper quartile =0.5200,
          upper whisker  =0.7692
        },
        ] coordinates {(0,0.20309051)(0,0.76923077)(0,0.10603829)(0,0.34626866)(0,0.16532258)(0,0.56716418)(0,0.57358491)(0,0.17500000)(0,0.29811321)(0,0.45575221)(0,0.46650124)(0,0.28633406)(0,0.41121495)(0,0.69444444)(0,0.14562002)(0,0.14772727)(0,0.67692308)(0,0.47286822)(0,0.07709751)(0,0.36117381)};
        \addplot+[mark = o,
        boxplot prepared={
          lower whisker  =0.2467,
          lower quartile =0.3368,
          median         =0.4350,
          upper quartile =0.5505,
          upper whisker  =0.7826
        },
        ] coordinates {(0,0.3562264)(0,0.7826087)(0,0.2866044)(0,0.4327323)(0,0.3392659)(0,0.5944444)(0,0.5737705)(0,0.3342906)(0,0.3840304)(0,0.4867359)(0,0.527227)(0,0.3937138)(0,0.5111111)(0,0.6533865)(0,0.2625087)(0,0.2930944)(0,0.6439024)(0,0.5132743)(0,0.2467357)(0,0.4372256)};
      \end{axis}
      % \node[above,font=\bfseries] at (current bounding box.north) {F1 Score};
      \end{tikzpicture}
