# Supplementary material for: A Flexible Model for Record Linkage
Source: arXiv:2407.06835 source file (2025-09-15)
Supplement: Supplementary file 7 [file FDR_SHIW.tex]

\begin{tikzpicture}[x=1pt,y=1pt]
      \begin{axis}
        [
        boxplot/draw direction=y,
        ymin=0,ymax=1,
        xtick={1,2,3,4},
        xticklabels={\textit{FlexRL}, \textit{Exchanger}, \textit{BRL}, Simplistic},
        cycle list={{black},{black},{black},{black}}
        ]
        \addplot+[mark = o,
        boxplot prepared={
          lower whisker  =0.1818,
          lower quartile =0.2806,
          median         =0.3486,
          upper quartile =0.4176,
          upper whisker  =0.5161
        },
        ] coordinates {(0,0.4285714)(0,0.1818182)(0,0.2629108)(0,0.3786408)(0,0.3809524)(0,0.2830189)(0,0.3200000)(0,0.3245033)(0,0.4423077)(0,0.3736264)(0,0.2781065)(0,0.3028169)(0,0.4065934)(0,0.1923077)(0,0.4472362)(0,0.4508197)(0,0.2441860)(0,0.3500000)(0,0.5161290)(0,0.3472222)};
        \addplot+[mark = o,
        boxplot prepared={
          lower whisker  =0.5776,
          lower quartile =0.7887,
          median         =0.8937,
          upper quartile =0.9435,
          upper whisker  =0.9610
        },
        ] coordinates {(0,0.9543168)(0,0.3809524)(0,0.9610140)(0,0.9339875)(0,0.9385027)(0,0.8239437)(0,0.7535211)(0,0.9420935)(0,0.9072165)(0,0.8683417)(0,0.8285256)(0,0.9327247)(0,0.6746988)(0,0.5776398)(0,0.9449772)(0,0.9598503)(0,0.6020408)(0,0.8246154)(0,0.9543224)(0,0.8801792)};
        \addplot+[mark = o,
        boxplot prepared={
          lower whisker  =0.1628,
          lower quartile =0.2453,
          median         =0.2809,
          upper quartile =0.3298,
          upper whisker  =0.4133
        },
        ] coordinates {(0,0.2923077)(0,0.2857143)(0,0.1627907)(0,0.2839506)(0,0.1800000)(0,0.2692308)(0,0.2549020)(0,0.3333333)(0,0.3361345)(0,0.2426471)(0,0.2480000)(0,0.1951220)(0,0.4133333)(0,0.2346939)(0,0.3263158)(0,0.3809524)(0,0.2826087)(0,0.2738095)(0,0.3703704)(0,0.2792793)};
        \addplot+[mark = o,
        boxplot prepared={
          lower whisker  =0.1818,
          lower quartile =0.5327,
          median         =0.6787,
          upper quartile =0.7773,
          upper whisker  =0.8484
        },
        ] coordinates {(0,0.7481323)(0,0.1818182)(0,0.8162450)(0,0.6659529)(0,0.7744083)(0,0.4540816)(0,0.4827586)(0,0.7802115)(0,0.7403599)(0,0.6170599)(0,0.5981132)(0,0.7132530)(0,0.5837104)(0,0.3834586)(0,0.8394535)(0,0.8058659)(0,0.3529412)(0,0.5827338)(0,0.8483675)(0,0.6914498)};
      \end{axis}
      % \node[above,font=\bfseries] at (current bounding box.north) {False Discovery Rate};
      \end{tikzpicture}
