# Supplementary material for: A Flexible Model for Record Linkage
Source: arXiv:2407.06835 source file (2025-09-15)
Supplement: Supplementary file 8 [file Sensitivity_SHIW.tex]

\begin{tikzpicture}[x=1pt,y=1pt]
      \begin{axis}
        [
        boxplot/draw direction=y,
        ymin=0,ymax=1,
        xtick={1,2,3,4},
        xticklabels={\textit{FlexRL}, \textit{Exchanger}, \textit{BRL}, Simplistic},
        cycle list={{black},{black},{black},{black}}
        ]
        \addplot+[mark = o,
        boxplot prepared={
          lower whisker  =0.1086957,
          lower quartile =0.2457298,
          median         =0.2826855,
          upper quartile =0.4511318,
          upper whisker  =0.7500000
        },
        ] coordinates {(0,0.268041237113402)(0,0.75)(0,0.24685534591195)(0,0.251968503937008)(0,0.174887892376682)(0,0.463414634146341)(0,0.521472392638037)(0,0.244604316546763)(0,0.282238442822384)(0,0.325949367088608)(0,0.438848920863309)(0,0.261213720316623)(0,0.388489208633094)(0,0.711864406779661)(0,0.140485312899106)(0,0.144086021505376)(0,0.631067961165049)(0,0.373563218390805)(0,0.108695652173913)(0,0.283132530120482)};
        \addplot+[mark = o,
        boxplot prepared={
          lower whisker  =0.2537634,
          lower quartile =0.3095743,
          median         =0.3558077,
          upper quartile =0.4015231,
          upper whisker  =0.4573171
        },
        ] coordinates {(0,0.280927835051546)(0,0.541666666666667)(0,0.35062893081761)(0,0.291338582677165)(0,0.360986547085202)(0,0.457317073170732)(0,0.429447852760736)(0,0.311750599520384)(0,0.35036496350365)(0,0.414556962025316)(0,0.384892086330935)(0,0.369393139841689)(0,0.388489208633094)(0,0.576271186440678)(0,0.307397959183673)(0,0.253763440860215)(0,0.378640776699029)(0,0.327586206896552)(0,0.292270531400966)(0,0.322289156626506)};        
        \addplot+[mark = o,
        boxplot prepared={
          lower whisker  =0.04106280,
          lower quartile =0.09632384,
          median         =0.23465516,
          upper quartile =0.40699467,
          upper whisker  =0.83333333
        },
        ] coordinates {(0,0.118556701030928)(0,0.833333333333333)(0,0.0566037735849057)(0,0.228346456692913)(0,0.0919282511210762)(0,0.463414634146341)(0,0.466257668711656)(0,0.100719424460432)(0,0.192214111922141)(0,0.325949367088608)(0,0.338129496402878)(0,0.174142480211082)(0,0.316546762589928)(0,0.635593220338983)(0,0.0816326530612245)(0,0.0838709677419355)(0,0.640776699029126)(0,0.350574712643678)(0,0.0410628019323672)(0,0.240963855421687)};
        \addplot+[mark = o,
        boxplot prepared={
          lower whisker  =0.5978495,
          lower quartile =0.6424742,
          median         =0.6642686,
          upper quartile =0.7086147,
          upper whisker  =0.7661871
        },
        ] coordinates {(0,0.608247422680412)(0,0.75)(0,0.650943396226415)(0,0.614173228346457)(0,0.683856502242152)(0,0.652439024390244)(0,0.644171779141104)(0,0.697841726618705)(0,0.737226277372263)(0,0.667721518987342)(0,0.766187050359712)(0,0.627968337730871)(0,0.661870503597122)(0,0.694915254237288)(0,0.719387755102041)(0,0.597849462365591)(0,0.640776699029126)(0,0.666666666666667)(0,0.661835748792271)(0,0.75)};
      \end{axis}
      % \node[above,font=\bfseries] at (current bounding box.north) {F1 Score};
      \end{tikzpicture}
