# Supplementary material for: A Flexible Model for Record Linkage
Source: arXiv:2407.06835 source file (2025-09-15)
Supplement: Supplementary file 9 [file suppl_tab_RLData500_Results.tex]

\begin{table}[!ht]
    \centering
    \begin{tabular}{ccccccc}
      \hline
      \noalign{\vskip\doublerulesep \vskip-\arrayrulewidth}
      \multicolumn{1}{c}{\textbf{Methods}} & \multicolumn{2}{c}{\textbf{Linked Records}} & \multirow{2}{*}{\textbf{FN}} & \multirow{2}{*}{\textbf{F1-Score}} & \multirow{2}{*}{\textbf{FDR}} & \multirow{2}{*}{\textbf{Sensitivity}} \\
      \cline{2-3}
      \noalign{\vskip\doublerulesep \vskip-\arrayrulewidth}
      \multicolumn{1}{c}{} & \textbf{TP} & \textbf{FP} & & & &  \\
      \hline
      \noalign{\vskip\doublerulesep \vskip-\arrayrulewidth}
      \textbf{\textit{FlexRL} with soundex} & $44$ & $0$ & $6$ & $.94$ & $0$ & $.88$ \\
      \textbf{\textit{FlexRL}} & $38$ & $0$ & $12$ & $.86$ & $0$ & $.76$ \\
      \textbf{\textit{Exchanger}} & $49$ & $0$ & $1$ & $.99$ & $0$ & $.98$ \\
      \textbf{\textit{BRL}} & $50$ & $1$ & $0$ & $.99$ & $.02$ & $1$ \\
      \textbf{Simplistic approach with soundex} & $20$ & $0$ & $30$ & $.57$ & $0$ & $.40$ \\
      \textbf{Simplistic approach} & $0$ & $0$ & $50$ & & & \\
      \hline
      \noalign{\vskip\doublerulesep \vskip-\arrayrulewidth}
    \end{tabular}
    \caption{Performance of the compared methods on the RLData500 data with 50 links.}
    \label{tab_RLdata500_results}
\end{table}
