# Supplementary material for: A Flexible Model for Record Linkage
Source: arXiv:2407.06835 source file (2025-09-15)
Supplement: Supplementary file 10 [file suppl_tab_RLData500_Story.tex]

\begin{table}[!ht]
    \centering
    \begin{tabular}{ccccccc}
        \hline
        \noalign{\vskip\doublerulesep \vskip-\arrayrulewidth}
        \multicolumn{2}{c}{\textbf{Registrations}} & \textbf{First name} & \textbf{Family name} & \textbf{Birth year} & \textbf{Birth month} & \textbf{Birth day} \\
        \hline
        \noalign{\vskip\doublerulesep \vskip-\arrayrulewidth}
        \multirow{3}{*}{\textbf{Data}} & \textbf{Unique} & $146$ & $108$ & $86$ & $12$ & $31$ \\
        & \textbf{Unique in encoded} & $114$ & $85$ &  &  &  \\
        & \textbf{Type} & character & character & numeric & numeric & numeric \\
        \cline{2-2}
        \noalign{\vskip\doublerulesep \vskip-\arrayrulewidth}
        \multirow{2}{*}{\textbf{True Links}} & \textbf{Agree} & $.68$ & $.68$ & $.84$ & $.92$ & $.80$ \\
        & \textbf{Agree in encoded} & $.92$ & $.88$ &  &  &  \\
        \hline
        \noalign{\vskip\doublerulesep \vskip-\arrayrulewidth}
    \end{tabular}
    \caption{Summary of the RLData500 data. Characteristics of the PIVs in their original format and with soundex encoding for names. Level of agreements among the 50 links referring to the same individuals. No missing value in the dataset.}
    \label{tab_RLdata500_story}
\end{table}
