# Supplementary material for: A Flexible Model for Record Linkage
Source: arXiv:2407.06835 source file (2025-09-15)
Supplement: Supplementary file 11 [file suppl_tab_SHIW_complete_results.tex]

\begin{table}[!ht]
    \centering
    \begin{tabular}{ccccccc}
      \hline
      \noalign{\vskip\doublerulesep \vskip-\arrayrulewidth}
      \multicolumn{1}{c}{\textbf{Methods}} & \multicolumn{2}{c}{\textbf{Linked Records}} & \multirow{2}{*}{\textbf{FN}} & \multirow{2}{*}{\textbf{F1-Score}} & \multirow{2}{*}{\textbf{FDR}} & \multirow{2}{*}{\textbf{Sensitivity}} \\
      \cline{2-3}
      \noalign{\vskip\doublerulesep \vskip-\arrayrulewidth}
      \multicolumn{1}{c}{} & \textbf{TP} & \textbf{FP} & & & & \\
      \hline
      \noalign{\vskip\doublerulesep \vskip-\arrayrulewidth}
      \textbf{\textit{FlexRL} (0.5)} & $2435$ & $6711$ & $3995$ & $.31$ & $.73$ & $.38$ \\
      \textbf{Simplistic approach} & $4318$ & $13807$ & $2112$ & $.35$ & $.76$ & $.67$\\
      \hline
      \noalign{\vskip\doublerulesep \vskip-\arrayrulewidth}
      \textbf{\textit{FlexRL} (0.6)} & $2266$ & $5438$ & $4164$ & $.32$ & $.71$ & $.35$\\
      \textbf{\textit{FlexRL} (0.7)} & $2091$ & $4490$ & $4339$ & $.32$ & $.68$ & $.33$\\
      \textbf{\textit{FlexRL} (0.8)} & $1941$ & $3749$ & $4489$ & $.32$ & $.66$ & $.30$\\
      \textbf{\textit{FlexRL} (0.9)} & $1788$ & $3080$ & $4642$ & $.32$ & $.63$ & $.28$\\
      \hline
      \noalign{\vskip\doublerulesep \vskip-\arrayrulewidth}
    \end{tabular}
    \caption{Performance of FlexRL on the complete SHIW data for several linkage probability threshold (superior to 0.5 to ensure a one-to-one assignment) and of the simplistic approach.}
    \label{tab_SHIWFull_results}
\end{table}
