# Supplementary material for: A Flexible Model for Record Linkage
Source: arXiv:2407.06835 source file (2025-09-15)
Supplement: Supplementary file 12 [file suppl_tab_SHIW_description.tex]

\begin{table}[!ht]
    \centering
    \begin{tabular}{cccccccc}
        \hline
        \multicolumn{2}{c}{\textbf{Registrations}} & \textbf{Sex} & \textbf{Birth year} & \textbf{Marital status} & \textbf{Regional code} & \textbf{Birth region} & \textbf{Education} \\
        \hline
        \noalign{\vskip\doublerulesep \vskip-\arrayrulewidth}
        \multirow{2}{*}{\textbf{Data}} & \textbf{Unique} & $2$ & $97$ & $4$ & $20$ & $20$ & $6$  \\
        & \textbf{Type} & categorical & categorical & categorical & categorical & categorical & categorical \\
        \cline{2-2}
        \noalign{\vskip\doublerulesep \vskip-\arrayrulewidth}
        \multirow{1}{*}{\textbf{True Links}} & \textbf{Agree} & $1$ & $.98$ & $.94$ & $1$ & $.94$ & $.77$ \\
        \hline
        \noalign{\vskip\doublerulesep \vskip-\arrayrulewidth}
    \end{tabular}
    \caption{Summary of the full SHIW data of 2016 and 2020. Characteristics of the PIVs and level of agreement among the 6 430 links referring to the same individuals. There are $5\%$ of missing value in birth region in both data sets.}
    \label{tab_SHIW_Story}
\end{table}
